# Supplementary material for: Modeling Long-Range Context for Concurrent Dialogue Acts Recognition
Source: arXiv:1909.00521 source file (2019-10-22)
Supplement: Supplementary file 1 [file appendix.tex]

\appendix
\section{Appendix}\label{sec:appendix}

\begin{figure*}[htb]
    \centering
\includegraphics[width=0.8\textwidth]{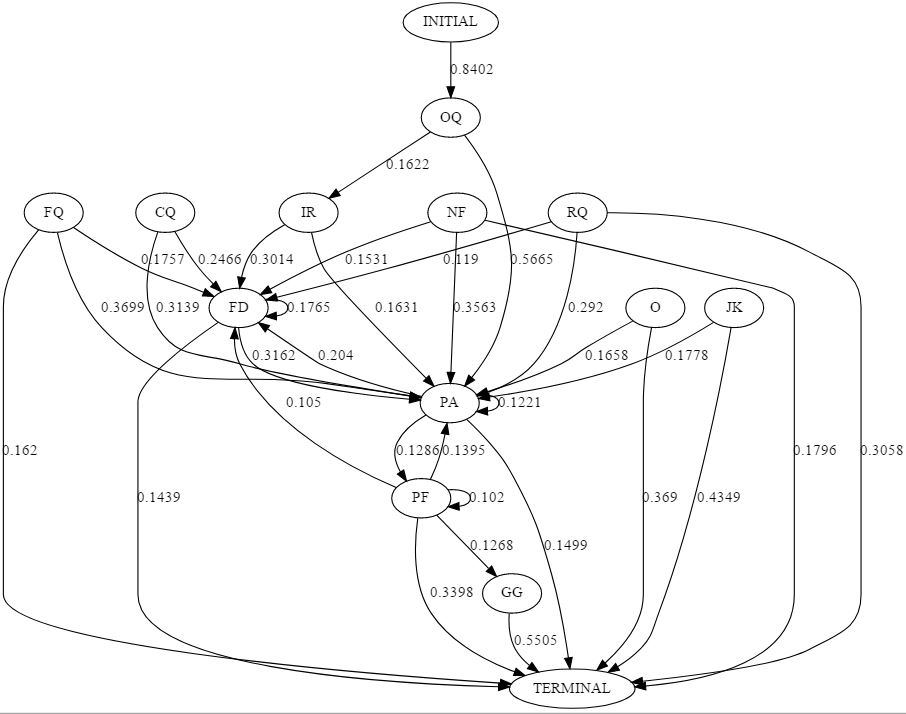}    \caption{Reproduced Markov chain for Dialogue Acts in MSDialog-Intent}
    \label{fig:msmarkovchain}
\end{figure*}

\begin{table*}[htb]
\small
\begin{tabular}{llllllllllllll}
\toprule
from\textbackslash{}to & CQ & FD & FQ & GG & IR & JK & NF & O & OQ & PA & PF & RQ & TERM. \\
\midrule
CQ & 5.3\% & 24.7\% & 4.4\% & 1.1\% & 7.1\% & 1.1\% & 3.6\% & 0.8\% & 0.5\% & \textbf{31.4\%} & 6.6\% & 3.9\% & 9.8\% \\
\hline
FD & 4.2\% & 17.7\% & 5.2\% & 2.9\% & 6.9\% & 1.6\% & 4.1\% & 1.1\% & 0.7\% & \textbf{31.6\%} & 6.3\% & 3.4\% & 14.4\% \\
\hline
FQ & 3.2\% & 17.6\% & 5.6\% & 0.8\% & 5.2\% & 1.5\% & 3.6\% & 0.8\% & 0.6\% & \textbf{37.0\%} & 4.8\% & 3.2\% & 16.2\% \\
\hline
GG & 1.0\% & 6.6\% & 3.3\% & 8.8\% & 0.3\% & 2.5\% & 3.3\% & 0.3\% & 1.0\% & 8.3\% & 4.0\% & 5.6\% & \textbf{55.1\%} \\
\hline
IR & 6.8\% & \textbf{30.1\%} & 7.2\% & 0.7\% & 7.0\% & 1.3\% & 5.4\% & 1.2\% & 1.2\% & 16.3\% & 9.6\% & 4.3\% & 8.9\% \\
\hline
JK & 2.5\% & 8.3\% & 2.5\% & 2.5\% & 3.2\% & 5.7\% & 3.8\% & 1.6\% & 0.6\% & 17.8\% & 3.2\% & 4.8\% & \textbf{43.5\%} \\
\hline
NF & 3.0\% & 15.3\% & 3.2\% & 1.4\% & 6.7\% & 2.5\% & 4.7\% & 1.4\% & 0.6\% & 35.6\% & 3.6\% & 4.0\% & 18.0\% \\
\hline
O & 1.6\% & 8.6\% & 3.2\% & 5.9\% & 3.2\% & 5.4\% & 5.9\% & 5.4\% & 0.5\% & 16.6\% & 3.7\% & 3.2\% & \textbf{36.9\%} \\
\hline
OQ & 6.2\% & 9.5\% & 2.7\% & 0.1\% & 16.2\% & 0.7\% & 0.8\% & 0.8\% & 1.2\% & \textbf{56.7\%} & 1.3\% & 2.6\% & 1.5\% \\
\hline
PA & 6.3\% & \textbf{20.4\%} & 9.3\% & 1.9\% & 3.7\% & 1.8\% & 8.6\% & 0.9\% & 1.4\% & 12.2\% & 12.9\% & 5.6\% & 15.0\% \\
\hline
PF & 1.7\% & 10.5\% & 4.4\% & 12.7\% & 2.0\% & 2.1\% & 2.8\% & 1.4\% & 0.8\% & 14.0\% & 10.2\% & 3.7\% & \textbf{34.0\%} \\
\hline
RQ & 3.6\% & 11.9\% & 2.4\% & 0.8\% & 5.5\% & 2.3\% & 2.9\% & 1.3\% & 1.0\% & \textbf{29.2\%} & 2.5\% & 6.1\% & 30.6\% \\
\hline
INIT. & 0.9\% & 7.4\% & 1.2\% &  & 2.5\% & 0.5\% & 2.4\% & 0.1\% & \textbf{84.0\%} & 0.5\% & 0.2\% & 0.4\% & \\
\bottomrule
\end{tabular}
\caption{\label{tab:Markovprob} \centering Transition probability (for each DA in the row, the probability of next DA in the column; each row sums up to 100\% and top probabilities are bolded)}
\end{table*}
